# Supplementary material for: Temporal Cascade Model for Analyzing Spread in Evolving Networks with Disease Monitoring Applications
Source: arXiv:2203.14925 source file (2022-03-28)
Supplement: Supplementary file 1 [file 07-appendix.tex]

\begin{appendices}
\section{Results on social network datasets}
\input{plots/table_socialNetwork}

\begin{figure}[tb]
\centering
\scalebox{0.5}{
\fbox{
$\qed$ \LARGE\emph{RSM}, \ \ \ $\triangle$ \LARGE\emph{ESM}
   \ \ \ \tikz \draw[black,fill=black] (0.5,0) circle (.5ex);  \LARGE\emph{ Max-Deg}  \ \ \ \tikz \draw[black] (0,0) circle (.5ex); \LARGE\emph{ Random}
 }
%   \ \ $\triangle$ \ \tikz \draw[black,fill=black] (0.5,0)  \LARGE\emph{ T-immunization}}
}
\begin{subfigure}{\textwidth}
    		\input{plots/different_timewindow_wikiVote} \\ \small{(e) wiki-Vote}
\end{subfigure} 
% \quad
\begin{subfigure}{\textwidth}
    		\input{plots/different_timewindow_citHepPH} \\ \small {(f) cit-HepPH} 
    % 		\small {(f) cit-HepPH}
\end{subfigure}
% \quad
\begin{subfigure}{\textwidth}
    		\input{plots/different_timewindow_socEpinions1}\\ \small {(g) soc-Epinions1}
    \end{subfigure}  
    \caption{\textit{Performance results against different number of time windows ($k$=50)}}
    \label{normalized_binary_success_rate}   
\end{figure}

\end{appendices}
